# Supplementary material for: CyRSoXS: A GPU-accelerated virtual instrument for Polarized Resonant Soft X-ray Scattering (P-RSoXS)
Source: arXiv:2209.13121 source file (2022-09-27)
Supplement: Supplementary file 1 [file appendix.tex]

\newpage
\begin{Notation*}{}
\begin{itemize}
    \item $\Vector{e}$ : Electric field (default: X direction, rotated in XY plane)
    \item $\Vector{k}$ : wave vector.
    \item $\Vector{s_1},\Vector{s_2}$ : Director / Orientation vector for biaxial case
    \item Thickness of morphology in Z direction
\end{itemize}
\end{Notation*}{}
\section{Rotation of $\Vector{k}$}

\begin{figure}[h!]
\centering
\tdplotsetmaincoords{60}{110}
% \begin{tikzpicture}[scale=3,tdplot_main_coords]
 
%   % variables

  \def\phivec{60}
 
%   % axes & vector
%   \coordinate (O) at (0,0,0);
%   \draw[thick,->] (0,0,0) -- (1,0,0) node[anchor=north east]{$y$};
%   \draw[thick,->] (0,0,0) -- (0,1,0) node[anchor=north west]{$z$};
%   \draw[thick,->] (0,0,0) -- (0,0,1) node[anchor=south]{$x$};
%   \tdplotsetcoord{P}{\rvec}{\thetavec}{\phivec}
%     \draw[-stealth,color=red] (O) -- (P) node[above right] {$\Vector{k}$};
 
%   % arcs
%   \draw[dashed, color=red] (O) -- (Pxy);
%   \draw[dashed, color=red] (P) -- (Pxy);
%   \tdplotdrawarc[<-]{(O)}{0.4}{\thetavec+10}{90}
%     {anchor=north}{$\theta$}
% %   \tdplotsetthetaplanecoords{\phivec}
% %   \tdplotdrawarc[->,tdplot_rotated_coords]{(0,0,0)}{0.4}{0.5}{\thetavec}
%     % {anchor=south west}{$\phi$}
% \end{tikzpicture}
\begin{tikzpicture}[scale=5,tdplot_main_coords]
    \coordinate (O) at (0,0,0);
    \begin{scope}[thick,->]
      \def\l{.8}
      \draw (O) -- (\l,0,0) node[pos=1.15]{$y$} ; 
      \draw (O) -- (0,\l,0) node[pos=1.1]{$z$} ; 
      \draw (O) -- (0,0,\l) node[right,pos=1.05]{$x$};
    
    %   \draw (O) -- (\l,0,0) node[pos=1.15]{$x$} ; 
    %   \draw (O) -- (0,\l,0) node[pos=1.1]{$y$} ; 
    %   \draw (O) -- (0,0,\l) node[right,pos=1.05]{$z$};
    \end{scope}
    % \begin{scope}[thick,->]
    %   \def\l{.8}
    %   \draw[dashed] (O) -- (0.5*\l,0.5*\l,0) node[pos=1.15]{$y$};
    %   \draw (O) -- (0,\l,0) node[pos=1.1]{$z$} ; 
    %   \draw (O) -- (0,0,\l) node[pos=1.05]{$x$};
    % \end{scope}
    \coordinate (P) at (0.4,0.6,0,0);
    \coordinate (A) at (0.6,0.9,0,0);
    \coordinate (B) at (0.9,-0.6,0,0);
    \coordinate (C) at (0,0.2,1,0);
    % \tdplotsetcoord{P}{\rvec}{\thetavec}{0}
    \draw[-stealth,color=red] (O) -- (P) node[right,pos=1.0]{$\Vector{k}$};
    \draw[dashed,->,thick,color=brown] (O) -- (A) node[pos=1.1]{$\Vector{k_{\parallel}}$};
    \draw[dashed,->,thick,color=brown] (O) -- (B) node[pos=1.1]{$\Vector{k_{\bot}}$};
    \draw[dashed,->,thick,color=brown] (O) -- (C) node[pos=1.1]{$\Vector{k_{e}}$};
    \tdplotdrawarc[<-]{(O)}{0.4}{\phivec}{90}{anchor=west}{$\theta$}
     \tdplotdrawarc[<-]{(O)}{0.9}{195}{200}{anchor=south}{$\phi$}
    
    \pgfmathsetmacro{\cubex}{0.3}
\pgfmathsetmacro{\cubey}{0.1}
\pgfmathsetmacro{\cubez}{0.3}
\begin{scope}[shift={(-0.3,-0.1,0)}]
\draw[blue,fill=none] (0,0,0) -- ++(-\cubex,0,0) -- ++(0,-\cubey,0) -- ++(\cubex,0,0) -- cycle;
\draw[blue,fill=none] (0,0,0) -- ++(0,0,-\cubez) -- ++(0,-\cubey,0) -- ++(0,0,\cubez) -- cycle;
\draw[blue,fill=none] (0,0,0) -- ++(-\cubex,0,0) -- ++(0,0,-\cubez) -- ++(\cubex,0,0) -- cycle;
\end{scope}
% \def\lcube{.2}
% % \begin{scope}[shift={(-\lcube/2.0,-\lcube/2.0,-\lcube/2.0)}]
% \foreach \x in{-\lcube/2,\lcube/2}
% {   \draw (\x,-\lcube/2 ,-\lcube/2) -- (\x,-\lcube/2 ,\lcube/2);
%     % \draw (\x ,0,\lcube) -- (\x ,\lcube,\lcube);
%     % \draw (\lcube,\x ,\lcube) -- (\lcube,\x ,0);
%     % \draw (\x ,\lcube,\lcube) -- (\x ,\lcube,0);
%     % \draw (\lcube,0,\x ) -- (\lcube,\lcube,\x );
%     % \draw (0,\lcube,\x ) -- (\lcube,\lcube,\x );
% }
% \end{scope}
% \end{tikzpicture}
    % \tdplotsetthetaplanecoords{\phivec}
    % \tdplotdrawarc[<-,tdplot_rotated_coords,blue]
    %     {(0,0,0)}{0.5}{\thetavec}{90}{anchor=south west}{$\phi$}

    % \draw[dashed, color=red] (O) -- (Pxy) -- (P) ;
    % \tdplotsetcoord{Pp}{.5}{90}{\phivec}
    % \draw[blue!30] (Pxy) -- (Pp);
\end{tikzpicture}
\caption{Figure demonstrating two basis of coordinate system. The original set of coordinate system is formed by ($x, y, z$) axis defined by $Q_C$ basis. The another set of coordinate system is defined by ($k_\parallel, k_\bot, k_e$) defined by $Q_K$ basis. The morphology (defined by blue lines) is defined in ($Q_C$) basis, whereas the basis $Q_K$ is formed by the vectors in such a way that $\Vector{e}$ and $\Vector{k}$ is always parallel to $\Vector{k_e}$ and $\Vector{k_\parallel}$ respectively.}
\end{figure}
 We need to define the new coordinate system relative to $\Vector{k}$.  The three coordinate system, thus defined are as follows:
\begin{itemize}
    \item $\Vector{q_{\parallel}}$ : Axis parallel to the $\Vector{k}$ and perpendicular to $\Vector{e}$.
    \item $\Vector{q_{\bot}}$ : Axis perpendicular to both $\Vector{k}$ and $\Vector{e}$.
    \item $\Vector{q_{e}}$ : Axis perpendicular to  $\Vector{k}$ and parallel to $\Vector{e}$.
\end{itemize}

\begin{remark}
The  axes  $\Vector{q_{\parallel}}$ , $\Vector{q_{\bot}}$ and $\Vector{q_{e}}$ are orthogonal to each other and forms the basis for 3D coordinate system.
\end{remark}

\begin{remark}
We consider $\Vector{e}$ to be rotated in XY plane and  $\Vector{k}$ is rotated accordingly to ensure $\Vector{e}\bot\Vector{k}$. The rotation of $\Vector{e}$ outside of XY plane is accomplished by rotation of the director vectors.
\end{remark}

The rotation matrix can be computed as:
\begin{equation}
\begin{split}
    \Tensor{R_x} & = \begin{bmatrix}
    1 & 0 & 0 \\
    0 & \cos(-\theta) & -\sin(-\theta) \\
    0 & \sin(-\theta) & \cos(-\theta)
    \end{bmatrix} \\
    \Tensor{R_z} & = \begin{bmatrix}
    \cos(\phi) &  -\sin(\phi) & 0\\
    \sin(\phi) & \cos(\phi) & 0\\
    0 & 0 & 1 \\
    \end{bmatrix}
\end{split}
\end{equation}
The three new axis can be rewritten in terms of the original basis as:

\begin{equation}
    \begin{split}
        \Vector{q_{\parallel}} & =\Tensor{R_z}\times\Tensor{R_x}  \times \begin{bmatrix} 0 \\ 0 \\ 1 \end{bmatrix}  = \begin{bmatrix}
        -\sin(\phi)\sin(\theta) \\ \cos(\phi)\sin(\theta) \\ \cos(\theta)
        \end{bmatrix} \\
       \Vector{q_{\bot}} & = \Tensor{R_z}\times\Tensor{R_x}  \times \begin{bmatrix} 0 \\ 1 \\ 0 \end{bmatrix}  = \begin{bmatrix}
        -\sin(\phi)\cos(\theta) \\ \cos(\phi)\cos(\theta) \\ -\sin(\theta)
        \end{bmatrix} \\
          \Vector{q_{e}} & = \Tensor{R_z}\times\Tensor{R_x} \times \begin{bmatrix} 1\\ 0 \\0 \end{bmatrix}  = \begin{bmatrix}
       \cos(\phi) \\ \sin(\phi) \\ 0
        \end{bmatrix} \\
    \end{split}
\end{equation}

\begin{Notation*}{}
\begin{itemize}
    \item The vector in original coordinate system ($Q_C$) is written as:
    \begin{equation*}
        q_x \UnitVector{c_x} + q_y \UnitVector{c_y} + q_z \UnitVector{c_z}
    \end{equation*}
    \item The  equivalent vector in the new basis ($Q_K$) is written as:
    \begin{equation*}
        q_1 \UnitVector{q_{\parallel}} + q_2 \UnitVector{q_\bot} + q_3 \UnitVector{q_e}
    \end{equation*}
\end{itemize}
\end{Notation*}
Thus any vector can be transformed from original basis to new basis as:
\begin{equation}
\begin{split}
    \begin{bmatrix}
    -\sin(\phi) \sin(\theta) & -\sin(\phi) \cos(\theta) & \cos(\phi) \\
    \cos(\phi)\sin(\theta)  & \cos(\phi) \cos(\theta) & \sin(\phi) \\
    \cos(\theta) & -\sin(\theta) & 0
    \end{bmatrix}
    \begin{bmatrix}
    q_1 \\ q_2 \\ q_3
    \end{bmatrix}
    =
    \begin{bmatrix}
    q_x \\ q_y \\ q_z
    \end{bmatrix}
    \\
    \begin{bmatrix}
    q_1 \\ q_2 \\ q_3
    \end{bmatrix}
    =
    \begin{bmatrix}
    -\sin(\phi)\sin(\theta) &   \cos(\phi) \sin(\theta) &  \cos(\theta)\\
    -\sin(\phi)\cos(\theta)  & \cos(\phi)\cos(\theta) & -\sin(\theta) \\
    \cos(\phi)&  \sin(\phi) & 0
    \end{bmatrix}
    \begin{bmatrix}
    q_x \\ q_y \\ q_z
    \end{bmatrix}
    \end{split}
\end{equation}

The resultant $\Vector{k}^\text{rot}$ can be calculated as:
\begin{equation}
    \Vector{k}^\text{rot} = \Tensor{R_z}\times \Tensor{R_x}  \times \begin{bmatrix}
    0 \\
    0 \\
    k
    \end{bmatrix}
\end{equation}
\begin{equation}
\begin{split}
    \Vector{k}^\text{rot} = & k_x^\text{rot} \UnitVector{c_x} + k_y^\text{rot} \UnitVector{c_y} + k_z^\text{rot} \UnitVector{c_z} \\
     = & -|\Vector{k}| \sin(\phi) \sin(\theta) \UnitVector{c_x} + |\Vector{k}|\cos(\phi) \sin(\theta) \UnitVector{c_y} + |\Vector{k}| \cos(\theta) \UnitVector{c_z}
\end{split}
\end{equation}
where:
\begin{equation*}
    \begin{split}
        k_x^\text{rot} = & -|\Vector{k}| \sin(\phi) \sin(\theta) \\
        k_y^\text{rot} = & |\Vector{k}|\cos(\phi) \sin(\theta) \\
        k_z^\text{rot} = & |\Vector{k}| \cos(\theta)
    \end{split}
\end{equation*}
% \begin{remark}
% We assume the rotation of $\Vector{k}$ to be in YZ plane. The rotation of $\Vector{k}$ outside of the YZ plane must be accompanied by the rotation of $\Vector{e}$ to ensure $\Vector{e} \bot \Vector{k}$. 

% The rotation of $\Vector{e}$  and $\Vector{k}$ outside of YZ plane is achieved by rotating the morphology's director vector $\Vector{s_1}$ and $\Vector{s_2}$ by an equivalent angle.
% \end{remark}
\begin{remark}
The morphology is defined in original basis. ($Q_C$).
\end{remark}

\begin{remark}
Rotated electric field $\Vector{e}^\text{rot}$ is defined by $\sin(\phi) \UnitVector{c_x} + \cos(\phi) \UnitVector{c_y} + 0\UnitVector{c_z}$. It can be verified that $\Vector{e}^\text{rot}\cdot\Vector{k}^\text{rot} = 0$ ensuring $\Vector{e}^\mathrm{rot} \bot \Vector{k}^\mathrm{rot}$.
\end{remark}

\subsection{Differential scattering cross section computation}
The differential scattering cross section is given by 
\begin{equation}
    [X(\Vector{q})]_{Q_K} = |k^2(\Tensor{I} - \UnitVector{r}\UnitVector{r})\cdot \Vector{p}(\Vector{q})|
\end{equation}
\subsubsection{In new Basis ($Q_K$)}
\begin{remark}
Recall that the FFT is calculated in the basis $Q_C$. In order to compute $X(\Vector{q})$ in the basis $Q_K$, we need to transform $\Vector{p(q)}$ from $Q_C$ to $Q_K$.
\end{remark}
\begin{equation}
    \begin{split}
        X(\Vector{q})_{Q_K} = & [k^2(\Tensor{I} - \UnitVector{r}\UnitVector{r})\cdot \Vector{p}(\Vector{q})]_{Q_K}
        \\  = &
        \begin{bmatrix}
        k^2 \Tensor{I} - 
         \begin{pmatrix}
         q_3 \\
         q_2 \\
         k + q_1
         \end{pmatrix}
         \begin{pmatrix}
         q_3 \quad q_2 \quad  k + q_1
         \end{pmatrix}
         \end{bmatrix}
         \cdot
         \begin{bmatrix}
         p_{q_e} \\
         p_{q_\bot}\\
         p_{q_\parallel}
         \end{bmatrix}
    \end{split}
    \label{eq: Rot:ScatterQK}
\end{equation}

where:
\begin{equation*}
    \begin{split}
        p_{q_e} & = p_{q_x} \cos(\phi) + p_{q_y} \sin(\phi) \\
        p_{q_\bot} & =  -p_{q_x} \sin(\phi) \cos(\theta) + p_{q_y} \cos(\phi) \cos(\theta)   - p_{q_z} \sin(\theta) \\
        p_{q_\parallel} & = -p_{q_x}\sin(\phi) \sin(\theta)  + p_{q_y} \cos(\phi) \sin(\theta)   + p_{q_z} \cos(\theta)\\
        q_3 &= q_x \cos(\phi) + q_y \sin(\phi) \\
        q_2 & = -q_x \sin(\phi) \cos(\theta) + q_y \cos(\phi) \cos(\theta)   - q_z \sin(\theta) \\
        q_1 &=-q_x\sin(\phi) \sin(\theta)  + q_y \cos(\phi) \sin(\theta)   + q_z \cos(\theta)
    \end{split}
\end{equation*}

\subsubsection{In the original basis $(Q_C)$}

\begin{equation}
    \begin{split}
        X(\Vector{q})_{Q_C} = &[k^2(\Tensor{I} - \Vector{r}\Vector{r})\cdot\Vector{p(q)}]_{Q_C} \\
        =&
        \begin{bmatrix}
        k^2 \Tensor{I} - 
         \begin{pmatrix}
         k_x^\text{rot} + q_x \\
         k_y^\text{rot} + q_y \\
         k_z^\text{rot} + q_z
         \end{pmatrix}
         \begin{pmatrix}
         k_x^\text{rot} + q_x \quad k_y^\text{rot} + q_y \quad  k_z^\text{rot} + q_z
         \end{pmatrix}
         \end{bmatrix}
         \begin{pmatrix}
         p_x \\ p_y \\p_z
         \end{pmatrix}
    \end{split}
    % \label{eq: Rot:Scatter}
\end{equation}
In order to transform $X(q)_{Q_C}$ to $X(q)_{Q_K}$:
\begin{equation}
    X(\Vector{q})_{Q_K} =
    \begin{bmatrix}
    \cos(\phi) & \sin(\phi) & 0 \\
    -\sin(\phi)\cos(\theta) & \cos(\phi)\cos(\theta) & -\sin(\theta)\\
    -\sin(\phi)\sin(\theta) & \sin(\phi)\cos(\theta) & \cos(\theta)
    \end{bmatrix}
    X(\Vector{q})_{Q_C}
    \label{eq: Rot:ScatterQC}
\end{equation}

\begin{remark}
We verified the equivalency of the ~\eqnref{eq: Rot:ScatterQK} and ~\eqnref{eq: Rot:ScatterQC} symbolically.
\end{remark}

\subsection{Projection on Ewalds sphere}
\begin{equation}
    \begin{split}
        |\Vector{k}^\text{out}| &= |\Vector{k}^\text{in}| = |k|\\
        | (k + q_1) \UnitVector{c_{\parallel}} + q_2 \UnitVector{c_{\bot}} + q_3 \UnitVector{c_{e}}| &= k\\
        \implies
        q_1 &= -k + \sqrt{k^2 - q_2^2 - q_3 ^2}
        \end{split}
        \label{eq: Rot:Ewalds}
\end{equation}

% \subsection*{\color{red}{Questions}}
% % {\color{blue}{
% \begin{enumerate}
%     \item Does the calculation makes sense? Is ~\eqnref{eq: Rot:Scatter} correct? Should it be in the new basis ($\Vector{q_\parallel}, \Vector{q_\bot}, \Vector{q_e})$ instead of $(\Vector{q_x}, \Vector{q_y}, \Vector{q_z})$?
%     \item How are the value of $q_1$ in ~\eqnref{eq: Rot:Ewalds} averaged? When there is no rotation of $\Vector{k}$, we have $q_z$ only. But when we have rotation of $\Vector{k}$, we get the component of $q_1$ in $z$ and $y$ direction. Should we take the components along $z$ or simply add full $q_1$  without taking any components?
%     \item Is the [$q_{max},q_{min}$] same in both dimension with rotation of $\Vector{k}$. The range of [$q_{max},q_{min}$] is  [$\frac{-\pi}{\text{PhysSize}}$,$\frac{\pi}{\text{PhysSize}}$] in both $q_x$ and $q_y$ without rotation.  But with rotation, [$q_{max},q_{min}$] becomes [$\frac{-\pi\cos(\theta)}{\text{PhysSize}}$,$\frac{\pi\cos(\theta)}{\text{PhysSize}}$] for $\Vector{q_2}$ and [$\frac{-\pi}{\text{PhysSize}}$,$\frac{\pi}{\text{PhysSize}}$] for $\Vector{q_1}$ in new basis. Is it correct?
%     \item For Ewalds projection, we used:
%     \begin{equation}
%         \Vector{k}^\text{\textbf{out}} = \Vector{k}^\text{\textbf{in}} + \Vector{q}
%     \end{equation}
%     But in paper Eq. 7, states:
%     \begin{equation}
%         \Vector{k}^\text{\textbf{out}} = \Vector{k}^\text{\textbf{in}} - \Vector{q}
%     \end{equation}
%     Is this discrepancy justified?
% \end{enumerate}
% % }}
